# Supplementary material for: A four-qubit germanium quantum processor
Source: arXiv:2009.04268 ancillary file (2020-09-09)
Supplement: Supplementary file 1 [file hendrickx_fourqubit_supplementary_materials.pdf]

## Supplementary Material: A four-qubit germanium quantum processor

N.W. Hendrickx,<sup>1,\*</sup>, W.I.L. Lawrie,<sup>1</sup>, M. Russ,<sup>1</sup>, F. van Riggelen,<sup>1</sup>, S.L. de Snoo,<sup>1</sup>, R.N. Schouten,<sup>1</sup>, A. Sammak,<sup>2</sup>, G. Scappucci,<sup>1</sup>, and M. Veldhorst<sup>1,†</sup>

<sup>1</sup>*QuTech and Kavli Institute of Nanoscience, Delft University of Technology, P.O. Box 5046, 2600 GA Delft, The Netherlands*

<sup>2</sup>*QuTech and Netherlands Organisation for Applied Scientific Research (TNO), Stieltjesweg 1, 2628 CK Delft, The Netherlands*

(Dated: September 9, 2020)

### MATERIALS AND METHODS

#### Device fabrication

The device was fabricated on a Ge/SiGe heterostructure with a 55-nm-deep buried quantum well, grown by RP-CVD as detailed in [1, 2]. Starting from a Si wafer, the heterostructure comprises a 1.6  $\mu\text{m}$  relaxed Ge layer; a 1  $\mu\text{m}$  step graded  $\text{Si}_{1-x}\text{Ge}_x$  layer with a final Ge composition of  $x = 0.8$ ; a 500 nm relaxed  $\text{Si}_{0.2}\text{Ge}_{0.8}$  buffer layer; the 16-nm-thick compressively strained Ge quantum well; a 55 nm  $\text{Si}_{0.2}\text{Ge}_{0.8}$  spacer layer and finally a sacrificial Si cap layer ( $< 2$  nm). We define ohmic contacts by electron beam lithography and subsequent etching of the oxidized Si cap layer and deposition of a 30 nm Al contact layer [3]. Electrostatic gates are defined in two layers (20 nm and 40 nm Ti/Pd respectively), separated from both the substrate and each other by 7 nm of ALD-grown  $\text{Al}_2\text{O}_3$ .

#### Experimental setup

Measurements are performed in a Bluefors dilution refrigerator with a base temperature of  $T_{\text{base}} = 20$  mK. We use battery powered voltage sources to bias the electrostatic gates. Additionally, coaxial lines are connected to all plunger and barrier gates through an on-PCB bias-tee, which can be pulsed using a Keysight M3202A arbitrary waveform generator. Plunger gates P2, P3, and P4 are furthermore connected to a vector source (Rohde&Schwarz SGS100A for P3/P4 and Keysight PSG E8257D for P2) through room-temperature diplexers with a stop band of  $f = 400 - 1500$  MHz. We modulate the qubit driving pulses using the quadrature modulation inputs and use multiple vector sources to be able to drive all qubit resonance lines to overcome the limited output bandwidth of 400 MHz of the AWGs. Qubits Q2 and Q4 are driven using the vector source connected to P3, Q1 is driven from gate P4, and Q3 is driven from gate P2.

The charge sensors are connected to a resonant tank circuit consisting of a in-house made niobium-titanium-nitride (NbTiN) kinetic inductor with an expected inductance of  $L = 2$   $\mu\text{H}$ . We apply a resonant RF-tone at  $f = 147.3$  MHz and  $f = 139.9$  MHz for sensor S1 and S2 respectively. The reflected signal is split using a directional coupler mounted to the mK-plate of the fridge and amplified by a cryogenic amplifier at the 4K stage. Next, the signal is demodulated using an in-house build demodulation setup and measured using a Keysight M3102A digitizer card. This is further detailed in Fig. S1 below.

The data in Figure 5 of the main text are normalized with respect to the readout visibility as obtained from a Rabi measurement. We find  $P_{Q1Q2, \text{ not blocked}} = 0.15$ ,  $P_{Q1Q2, \text{ blocked}} = 0.78$ ,  $P_{Q3Q4, \text{ not blocked}} = 0.10$ , and  $P_{Q3Q4, \text{ blocked}} = 0.93$ .

#### Virtual gate matrices

In order to map out the transition lines of all four quantum dots in a single measurement, we define the following virtual gates [4] as linear combination of the physical gates  $P_1$ - $P_4$ , as well as the sensor plunger gates  $P_{S1}$  and  $P_{S2}$ .

We write:

$$\begin{pmatrix} P_1 \\ P_2 \\ P_3 \\ P_4 \\ P_{S1} \\ P_{S2} \end{pmatrix} = \begin{pmatrix} 1 & 1 \\ -1 & 1 \\ 0.75 & 1 \\ -0.75 & 1 \\ -0.1 & -0.4 \\ -0.05 & -0.51 \end{pmatrix} \begin{pmatrix} e_{1234} \\ U_{1234} \end{pmatrix}$$

with  $e_{1234} = \Delta(P_1 - P_2 + 0.75P_3 - 0.75P_4)$  and  $U_{1234} = \Delta(P_1 + P_2 + P_3 + P_4)$  the virtual gates used in Fig. 1C of the main text.

In addition, we define a virtual gate system to allow independent control of the different interdot couplings and quantum dot detuning and on-site energy and write:

$$\begin{pmatrix} P_1 \\ P_2 \\ P_3 \\ P_4 \\ B_{12} \\ B_{34} \\ B_{23} \\ B_{41} \\ P_{S1} \\ P_{S2} \end{pmatrix} = \begin{pmatrix} 1.2600 & 0.7400 & 0.3100 & -0.1700 & -0.5500 & 0 & 0 & -0.4900 \\ -1.3900 & 0.6100 & -0.3600 & -0.3600 & -1.0300 & 0 & -0.6000 & 0 \\ 0.2800 & -0.2800 & 1.3900 & 0.6100 & 0 & -0.4700 & -0.6000 & 0 \\ -0.3000 & -0.3000 & -1.3900 & 0.6100 & 0 & -0.9100 & 0 & -0.9200 \\ 0 & 0 & 0 & 0 & 1.0000 & 0 & 0 & 0 \\ 0 & 0 & 0 & 0 & 0 & 1.0000 & 0 & 0 \\ 0 & 0 & 0 & 0 & 0 & 0 & 1.0000 & 0 \\ 0 & 0 & 0 & 0 & 0 & 0 & 0 & 1.0000 \\ -0.0900 & -0.1500 & 0.0100 & -0.0300 & 0 & 0 & 0 & 0 \\ 0 & 0 & -0.0900 & -0.1500 & 0 & 0 & 0 & 0 \end{pmatrix} \begin{pmatrix} e_{12} \\ U_{12} \\ e_{34} \\ U_{34} \\ vB_{12} \\ vB_{34} \\ vB_{23} \\ vB_{41} \end{pmatrix}$$

with  $e_{mn}$  the detuning voltage and  $U_{mn}$  the voltage controlling the on-site energy of quantum dots  $m$  and  $n$ ,  $vB_{mn}$  the virtual barrier gate controlling the coupling between quantum dots  $m$  and  $n$ , and  $P_n$ ,  $B_{mn}$  and  $P_{S1-2}$  the various physical gates.

### Shift in Rabi frequency due to exchange

When exchange interaction is present in the quantum dot system, the energy levels of the qubit are modified and the qubit basis states hybridize. Conditional driving of the spin states is a direct consequence of the shift of the energy levels, which allows for controlled multi-qubit gates as previously employed to drive two-qubit gates [5–8]. The hybridization of the qubit states on the other hand gives rise to conditional Rabi frequencies that also depend on the strength of the exchange interaction [8]. Furthermore, the exchange interaction can become anisotropic in the presence of spin-orbit coupling [9]. When only considering the exchange interaction between neighboring quantum dots, a general Hamiltonian can be written for the four quantum dots in the (1,1,1,1) charge regime as:

$$H = \sum_{\langle i,j \rangle} \mathbf{S}_i \cdot \overline{\mathcal{J}}_{ij} \mathbf{S}_j + \sum_{i=1}^4 (\mathcal{B} + \mathcal{B}_{ac} \cos(2\pi f t + \phi)) \cdot \mathbf{S}_i, \quad (1)$$

where the first sum runs along every neighboring quantum dot pair  $\langle i,j \rangle$  with the corresponding tensorial exchange interaction  $\overline{\mathcal{J}}_{ij}$ . We note that the term  $\mathcal{B}$  consists of both the Zeeman effect due to the external magnetic field, and the contribution due to the spin-orbit interaction. We also explicitly separate the static Zeeman interaction from the field induced by the electric driving.

We take  $\mathcal{D}$  to be the unitary matrix which diagonalizes Hamiltonian (1) for  $\mathcal{B}_{ac} = 0$ , e.g.,  $\mathcal{D}^\dagger H(\mathcal{B}_{ac} = 0) \mathcal{D} = \mathbf{1}$ . Now, the effective Rabi amplitude between the eigenstates of the undriven Hamiltonian  $|\xi\rangle$  and  $|\zeta\rangle$  in the adiabatic limit of exchange is given by:

$$\Omega_{|\xi\rangle \rightarrow |\zeta\rangle} = \frac{1}{4} \langle \xi | \mathcal{D}^\dagger \mathcal{B}_{ac} \mathcal{D} | \zeta \rangle, \quad (2)$$

where the prefactor 1/4 is coming from the spin and the rotating wave approximation. Therefore, the Rabi amplitude depends on the exact form of the exchange interaction, as well as which transition is driven.

### Fitting of the two-qubit decay data

In order to extract the decay time scale in Fig. 4D of the main text, we fit the exchange interaction data to the model function  $P = A \cos(2\pi(f_0 + \delta x)t + \phi_0) \exp(-t/\tau) + y_0$ , with amplitude  $A$ , frequency  $f_0$ , phase offset  $\phi_0$ , and offset  $y_0$ . We note that we allow for a small linear shift of the precession frequency  $\delta$ , typically of size  $\delta = 10 \text{ MHz}/\mu\text{s}$ , as a result of pulse imperfections in these relatively large and extended exchange pulses. We observe a small creep towards the final pulse amplitude to be present, most likely caused by the skin effect in the coaxial lines, explaining the small observed frequency shift throughout the experiment. The data for the situation with no exchange present is fitted to the exponential decay  $P = \exp(-t/\tau) + y_0$ , from which we deduce the decay time scale  $\tau$ .

## SUPPLEMENTARY FIGURES

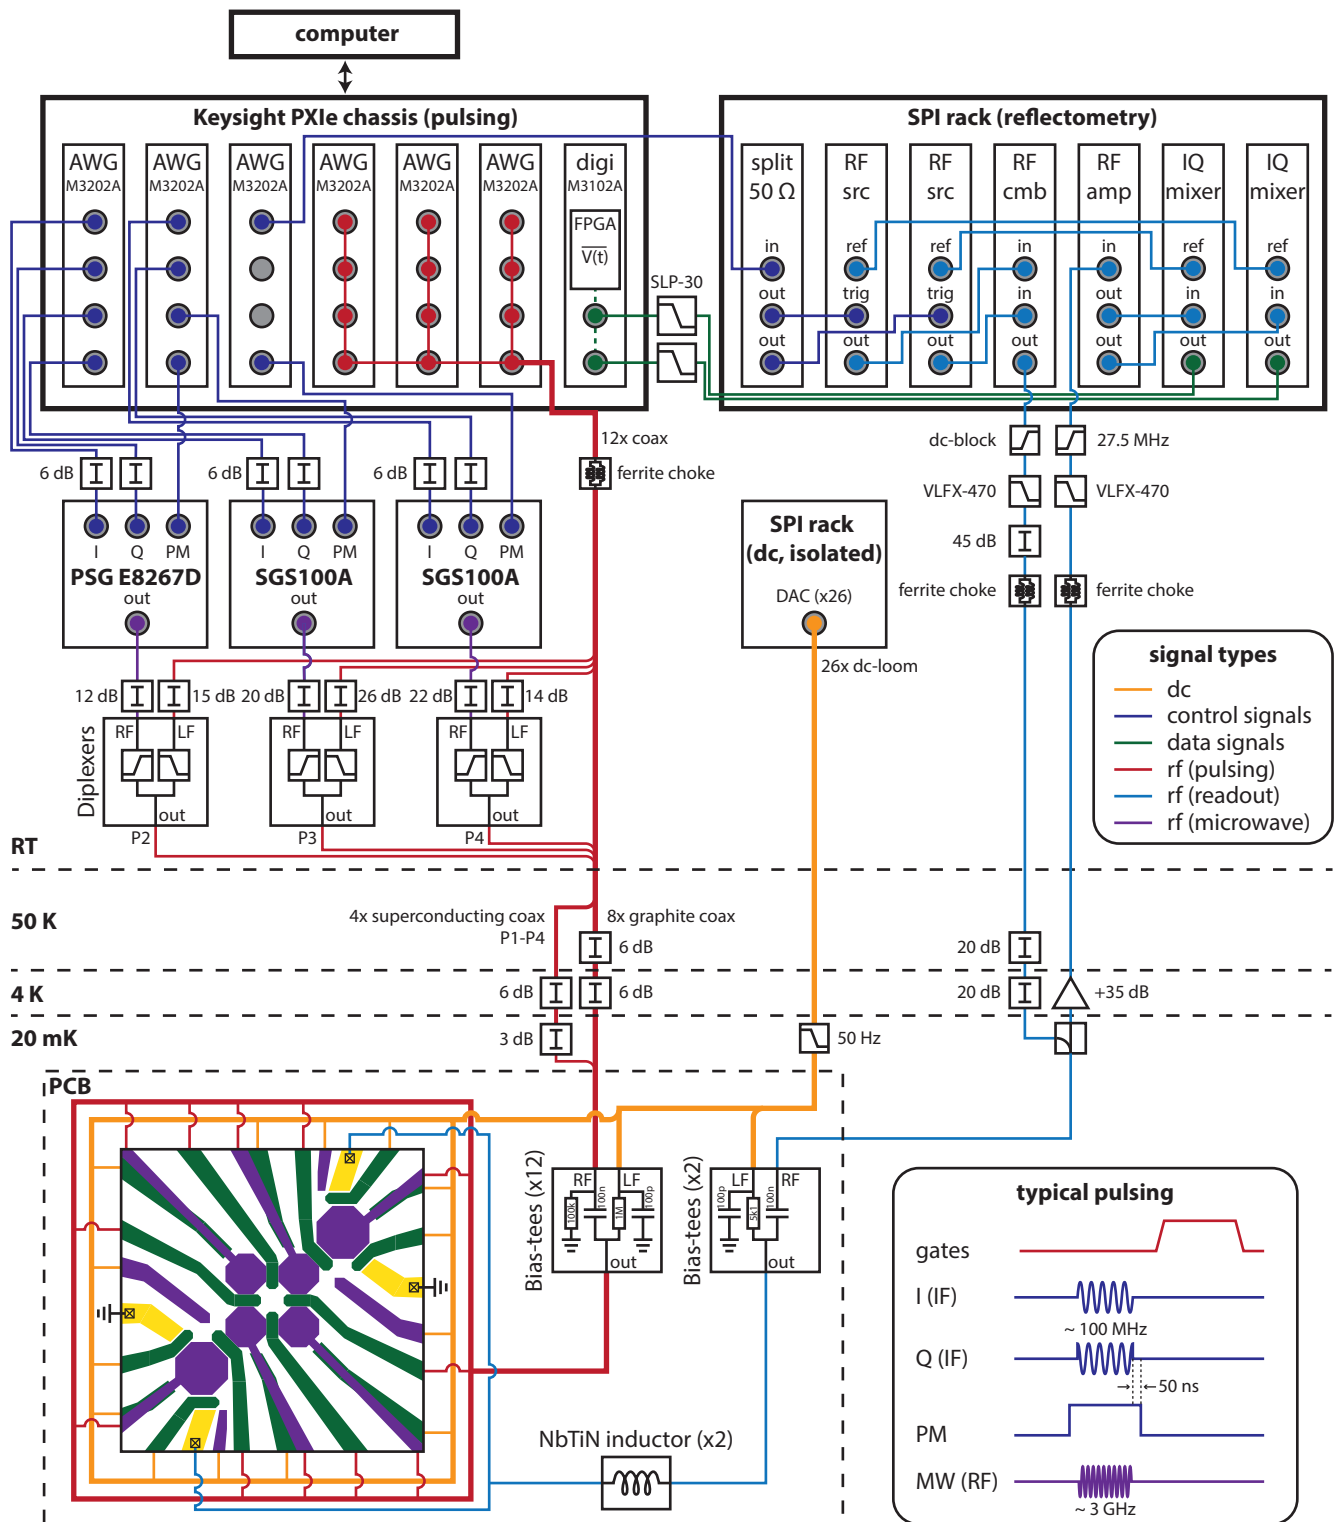

Figure S1. (*Previous page*) **Schematic of the measurement set-up** The sample is bonded to a printed circuit board (PCB) mounted to the cold finger of a dilution refrigerator. DC voltages (orange) are applied to the gates using galvanically isolated digital-to-analog converters (DACs) through lines filtered at the mixing chamber stage of the refrigerator. Voltage pulses (red) are applied to the same gates using Keysight M3202A arbitrary waveform generators (AWGs). The signals pass through an ferrite common mode choke and are attenuated at different stages of the fridge and are combined with the DC signal using on-PCB bias-tees. The microwave excitation used for spin resonance is generated by three separate vector sources and is combined with the AWG signal on plungers P2, P3, P4 through room temperature diplexers with pass bands dc-400 MHz and 1.5-10 GHz. The output of the vector sources is modulated by quadrature modulation using signals generated on the AWGs (dark blue). By applying sine waves with a phase difference of  $\pi/2$  to the in-phase (I) and quadrature (Q) inputs of the vector source, a single-sideband signal with controllable amplitude, frequency, phase and duration is acquired. Additionally, we apply a pulse modulation (PM) envelope around the microwave pulses to improve the microwave suppression to a total of -120 dB. Using an in-house built reflectometry set-up, we generate (RF src) two microwave tones resonant with the tank circuit on the PCB (light blue). The RF sources are pulse modulated by a trigger generated on the AWG, to mute the sources during qubit manipulation. The signals are combined (RF cmb), filtered and attenuated before reaching a directional coupler at the mixing chamber stage. Here, the signal propagates through two on-PCB bias-tees to the two NbTiN resonators, which form the tank circuits. The reflected signal is then split off and amplified by 35 dB at the 4K stage of the fridge using a CITLF3 cryogenic amplifier. The signal is amplified again at room temperature (RF amp) after which it is demodulated separately at both of the carrier frequencies to retrieve the charge sensor signal. After filtering the signal, it is recorded and temporally averaged using the FPGA in the digitizer to reduce the amount of data transferred to the computer.

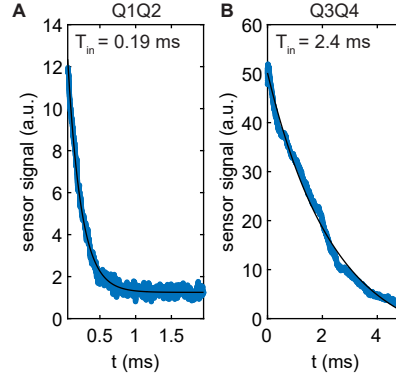

Figure S2. **Decay of the readout signal at the readout point (A-B)** We measure the difference in charge sensor signal between the blocked and non-blocked states as a function of the measurement time at the readout point. An exponential decay can be observed related to the tunnel time  $T_{in}$  of Q2 (Q4) to the reservoir for the Q1Q2 (A) and Q3Q4 (B) readout system respectively.

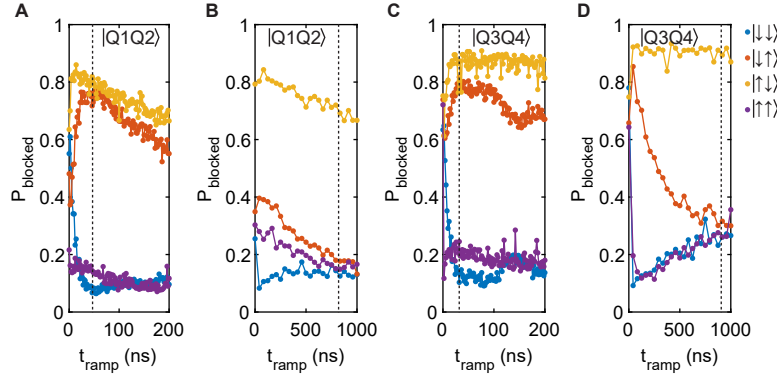

Figure S3. **Readout visibility of the different two-qubit states. (A-D)** We vary the ramp time between the manipulation phase and the readout phase and measure the blocked state probability of the four different two qubit basis states by applying preparation  $\pi$  pulses to the relevant qubits, both for the Q1Q2 readout system (A,B) and the Q3Q4 readout system (C,D). By increasing the interdot coupling during the readout and elongating the ramp between the manipulation and readout point, we can switch between a parity readout (A,C) and a single state readout (B,D). The dashed line corresponds to the optimized readout ramp time used for the measurements in this manuscript.

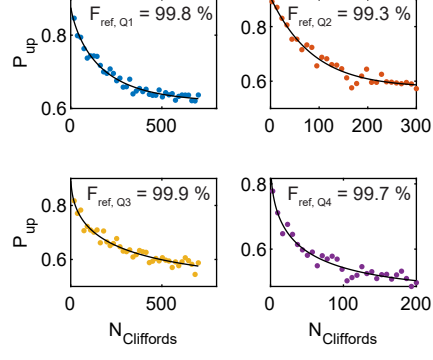

Figure S4. **Randomized benchmarking of the Clifford group** We quantify the quality of the single qubit gates by performing randomized benchmarking of the single-qubit Clifford group [10]. The decay curve of the qubit state is measured as a function of the number of Clifford gates applied. Each data point consists of 1000 single shots for 30 different randomly selected Clifford sequences with length  $N_{\text{Cliffords}}$ . The decay is fitted to  $P_{\text{up}} = a \exp(-(N_{\text{Cliffords}}/m)^\alpha) + y_0$ , with  $a$  the initial spin-up probability,  $m$  the decay parameter,  $\alpha$  the decay power and  $y_0$  an offset.  $F_{\text{ref}} = 1 - \frac{m}{2 \cdot 1.875}$  is extracted based on the average single qubit gate length of  $1/1.875$  Clifford gates.

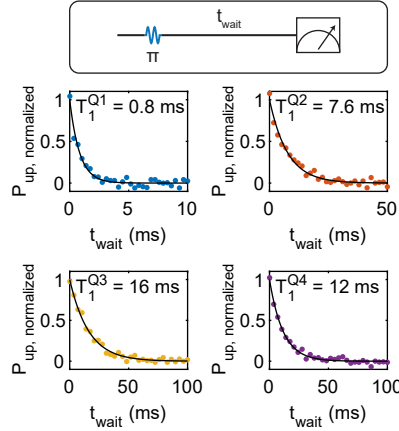

Figure S5. **Spin relaxation times of the different qubits** The spin relaxation time  $T_1$  is measured at the manipulation point by applying a  $\pi_X$ -pulse separated by a waiting time  $t_{\text{wait}}$  from the readout phase, as illustrated in the schematic on top. By fitting the normalized spin-up fraction to  $P = \exp(-t_{\text{wait}}/T_1)$ , we find spin relaxation times of  $T_{1,Q1} = 0.8$  ms,  $T_{1,Q2} = 7.6$  ms,  $T_{1,Q3} = 16$  ms, and  $T_{1,Q4} = 12$  ms for Q1-Q4 respectively.

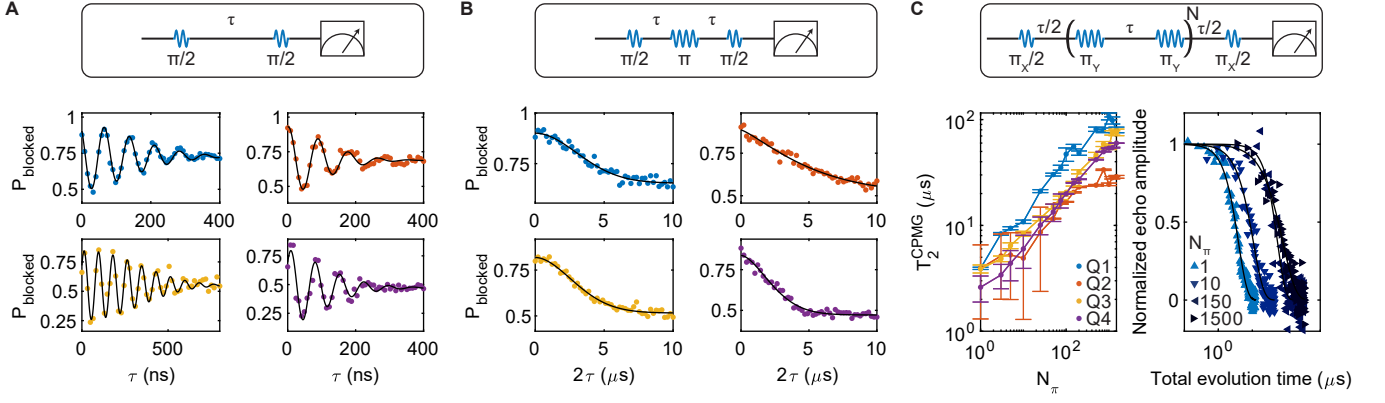

Figure S6. **Ramsey, Hahn echo and Carr-Purcell-Meiboom-Gill (CPMG) measurements on the different qubits.** (A) The phase coherence time  $T_2^*$  is measured using a Ramsey sequence consisting of two  $X(\pi/2)$ -pulses separated by a waiting time  $\tau$  as illustrated in the schematic on top. By fitting the data to  $P = \cos(2\pi\Delta f\tau + \phi_0) \exp(-(\tau/T_2^*)^\alpha)$ , with  $\Delta f$  the frequency detuning,  $\phi_0$  a phase offset and  $\alpha$  the power of the decay, we find spin dephasing times of  $T_{2,Q1}^* = 201$  ns,  $T_{2,Q2}^* = 146$  ns,  $T_{2,Q3}^* = 445$  ns, and  $T_{2,Q4}^* = 150$  ns for Q1-Q4 respectively. (B) Using an additional  $X(\pi)$ -pulse, low-frequency fluctuations of the qubit resonance frequency can be echoed out, allowing to probe the Hahn-echo decay time  $T_2^{\text{Hahn}}$ . Fitting the data to  $P = \exp(-(\tau/T_2^{\text{Hahn}})^\alpha)$ , we find Hahn echo times of  $T_{2,Q1}^{\text{Hahn}} = 4.3\mu\text{s}$ ,  $T_{2,Q2}^{\text{Hahn}} = 5.5\mu\text{s}$ ,  $T_{2,Q3}^{\text{Hahn}} = 3.8\mu\text{s}$ , and  $T_{2,Q4}^{\text{Hahn}} = 2.9\mu\text{s}$ . (C) Using a CPMG sequence of repeated  $Y(\pi)$  pulses, we can increase the echo bandwidth and extend the phase coherence to over  $T_{2,Q1}^{\text{CPMG}} > 100\mu\text{s}$ . The phase coherence can be observed to increase with the amount of refocusing pulses (left), with exemplary decay traces for Q1 plotted in the right panel.

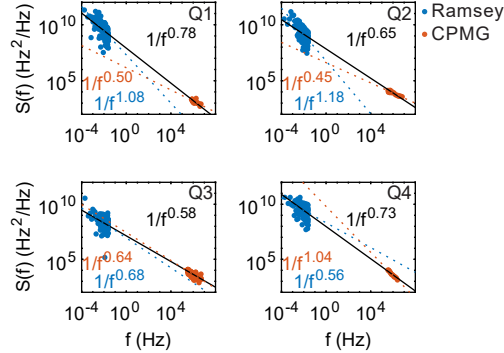

Figure S7. **Noise spectroscopy using Ramsey and CPMG measurements.** We measure the effective noise spectrum acting on the qubit, both tracing the resonance frequency using repeated Ramsey measurements [11] (in blue), as well as by using the filter function of a dynamical decoupling measurement [12, 13] (in red). Dashed blue and red lines are fits to the Ramsey and CPMG data respectively. The black line is a fit to the combined dataset, where the weight of both sets is normalized for the amount of data points. The effective noise can be observed to increase towards low frequencies, consistent with the upwards trend of  $T_2^{\text{CPMG}}$  observed in Fig. S1c. The effective charge noise measured in this heterostructure is  $S_{\text{cn}}(f) = 6\mu\text{V}/\sqrt{\text{Hz}}$  at 1 Hz [2]. Combining this with a typical resonance frequency slope of  $df/dV = 5\text{ MHz/mV}$  [14], results in an effective resonance frequency noise power of  $S(f) = 9 \cdot 10^8\text{ Hz}^2/\text{Hz}$ , comparable to what is observed experimentally, suggesting coherence is limited by charge noise in our system.

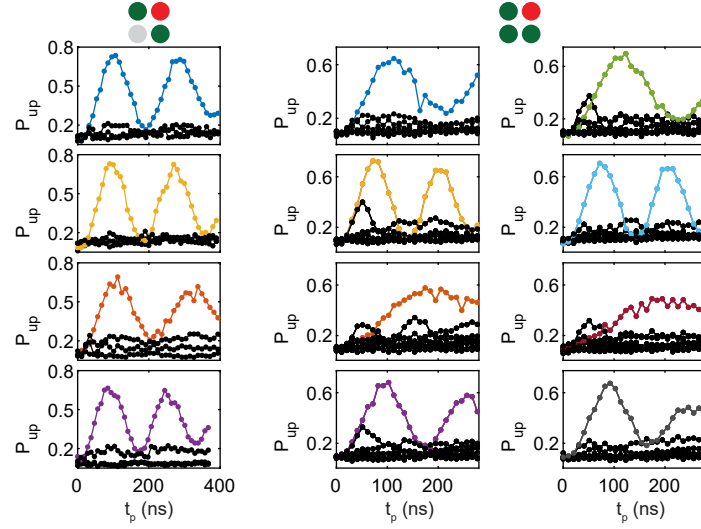

Figure S8. **Driving of all resonance lines of the coupled three and four qubit system.** (A) Both the coupling between Q2 and Q1 as well as Q2 and Q3 are enabled, using the respective virtual barrier gates. This splits the resonance line in four, as shown in Fig. 3 of the main text. Driving each of the separate lines, results in the conditional rotation of Q2 depending on the states of Q1 and Q3. We measure the spin up probability after driving each of the four resonance lines for time  $t_p$ , for all four permutations of the Q1 and Q3 basis states as initial state, following the color scheme of Fig. 3 in the main text. The driving power is adjusted for each of the transitions to synchronize the  $\pi$ -rotation times, with  $a_{f1} = 330$  mV,  $a_{f2} = 500$  mV,  $a_{f3} = 280$  mV, and  $a_{f4} = 400$  mV, for  $f1 - 4$  from top to bottom. (B) Similarly, by additionally opening up the coupling between Q3 and Q4 as well, the resonance line splits in four and we can drive all separate lines individually. The eight lines are driven using the same microwave power in this figure and a strong difference in rotation frequencies can be observed for the different transitions. This also results in a small off-resonant driving effect for some of the lines.

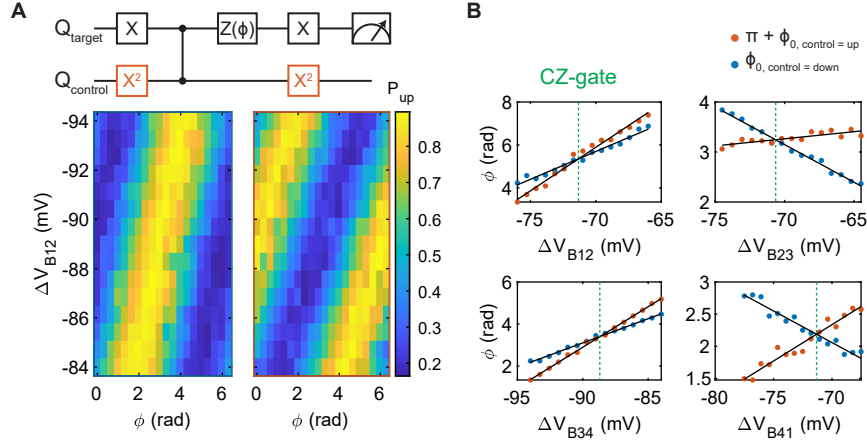

Figure S9. **Tuning of the CZ-gates.** (A-B) The CZ-gates between all four qubit pairs are tuned using a Ramsey sequence (analogous to Fig. 4 of the main text), where the spin-up probability is measured as a function of the phase  $\phi$  of the final  $\pi/2$  pulse as well as the depth of the exchange pulse  $V_{Bmn}$ , with  $m$  and  $n$  the relevant qubits (A). We choose to tune the height of the voltage pulse rather than its length, due to the limited temporal resolution of the exchange pulses (1 ns). The acquired phase  $\phi_0$  is obtained by fitting each line to  $P = A \cos(\phi + \phi_0) + y_0$ , with  $A$  the visibility and  $y_0$  an offset. A CZ-gate is achieved when the difference in acquired phase is exactly  $\Delta\phi = \pi$ , for the situation where the control qubit is  $|\downarrow\rangle$  (blue) compared to  $|\uparrow\rangle$  (orange). The barrier gate voltage at which this occurs is obtained from the intersection of two locally linear fits to the extracted acquired phase (B).

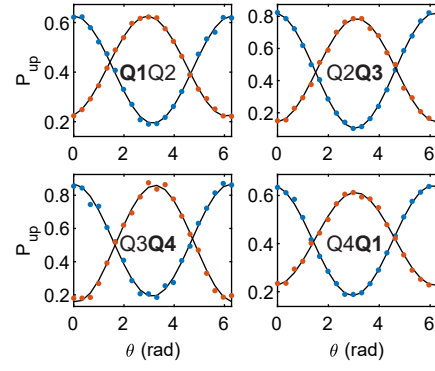

Figure S10. **CZ-gates between the four qubit pairs.** The CZ-gates between all four qubit pairs probed by a Ramsey sequence using the inverse qubits as target and control as compared to the data in Fig. 4B of the main text. The target qubit is marked in bold.

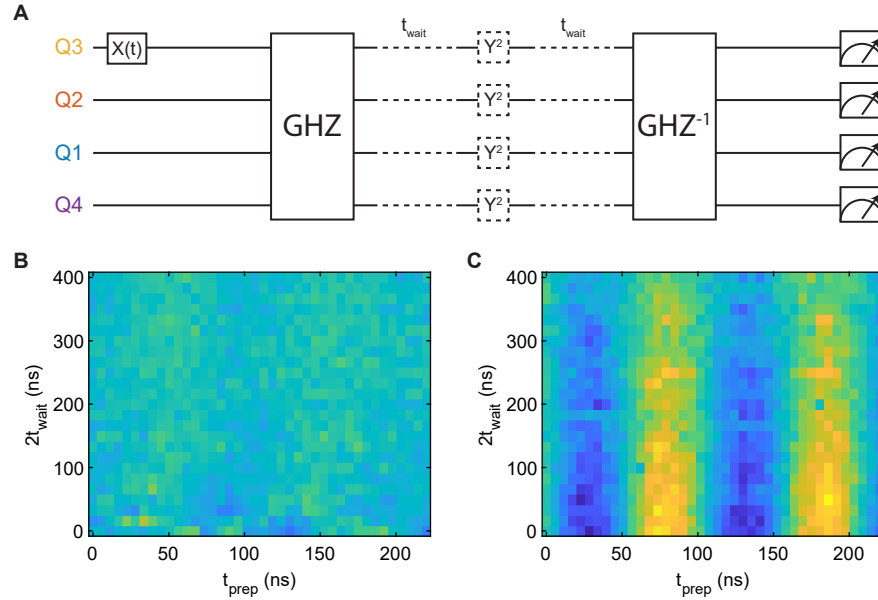

Figure S11. **Time evolution of the four-qubit GHZ state.** (A) Circuit diagram of the experiments performed in panels B-C. We first apply a preparation pulse to Q3 and then generate a four qubit GHZ-state analogous to Fig. 5 in the main text. Next we let the entangled system evolve for time  $t_{\text{wait}}$ , then apply an optional  $Y^2$  decoupling pulse and finally disentangle the GHZ-state again. (B-C) We vary both the waiting time and preparation time  $t_{\text{prep}}$  and plot the spin-up fraction of Q3 in the case without (B) and with (C) decoupling pulse. It can be clearly observed that without the echo pulse, the system has fully decohered at the end of the algorithm. However, by applying the decoupling pulse, the coherence of the entangled system can be maintained for a prolonged time scale, with a characteristic decay time of  $\tau = 390$  ns.

| target | transition                                                | control | $t_{\pi,\text{control}}$ (ns) | $t_{\pi,\text{target}}$ (ns) |
|--------|-----------------------------------------------------------|---------|-------------------------------|------------------------------|
| 1      | $ \downarrow\downarrow\rangle- \downarrow\uparrow\rangle$ | 2       | 67                            | 85                           |
| 1      | $ \downarrow\uparrow\rangle- \uparrow\uparrow\rangle$     | 2       | 67                            | 95                           |
| 1      | $ \downarrow\downarrow\rangle- \downarrow\uparrow\rangle$ | 4       | 61                            | 104                          |
| 1      | $ \downarrow\uparrow\rangle- \uparrow\uparrow\rangle$     | 4       | 61                            | 108                          |
| 2      | $ \downarrow\downarrow\rangle- \downarrow\uparrow\rangle$ | 1       | 45                            | 105                          |
| 2      | $ \downarrow\uparrow\rangle- \uparrow\uparrow\rangle$     | 1       | 41                            | 105                          |
| 2      | $ \downarrow\downarrow\rangle- \downarrow\uparrow\rangle$ | 3       | 38                            | 113                          |
| 2      | $ \downarrow\uparrow\rangle- \uparrow\uparrow\rangle$     | 3       | 38                            | 100                          |
| 3      | $ \downarrow\downarrow\rangle- \downarrow\uparrow\rangle$ | 2       | 65                            | 53                           |
| 3      | $ \downarrow\uparrow\rangle- \uparrow\uparrow\rangle$     | 2       | 65                            | 83                           |
| 3      | $ \downarrow\downarrow\rangle- \downarrow\uparrow\rangle$ | 4       | 49                            | 83                           |
| 3      | $ \downarrow\uparrow\rangle- \uparrow\uparrow\rangle$     | 4       | 45                            | 68                           |
| 4      | $ \downarrow\downarrow\rangle- \downarrow\uparrow\rangle$ | 1       | 45                            | 105                          |
| 4      | $ \downarrow\uparrow\rangle- \uparrow\uparrow\rangle$     | 1       | 45                            | 120                          |
| 4      | $ \downarrow\downarrow\rangle- \downarrow\uparrow\rangle$ | 2       | 38                            | 68                           |
| 4      | $ \downarrow\uparrow\rangle- \uparrow\uparrow\rangle$     | 2       | 38                            | 74                           |

Table S1. Driving times used in Fig. 2 of the main text.

| two-qubit system | $t_{\text{ramp}}$ (ns) | $t_{\text{gate}}$ (ns) |
|------------------|------------------------|------------------------|
| Q1Q2             | 3                      | 6                      |
| Q2Q3             | 10                     | 4                      |
| Q3Q4             | 10                     | 5                      |
| Q4Q1             | 3                      | 6                      |

Table S2. CZ gate details.

- 
- [1] A. Sammak, *et al.*, *Advanced Functional Materials* **29**, 1807613 (2019).
  - [2] M. Lodari, *et al.*, *arXiv: 2007.06328 [cond-mat]* (2020).
  - [3] N. W. Hendrickx, *et al.*, *Nature Communications* **9**, 2835 (2018).
  - [4] T. Hensgens, *et al.*, *Nature* **548**, 70 (2017).
  - [5] M. Veldhorst, *et al.*, *Nature* **526**, 410 (2015).
  - [6] T. F. Watson, *et al.*, *Nature* **555**, 633 (2018).
  - [7] D. M. Zajac, *et al.*, *Science* **359**, 439 (2018).
  - [8] M. Russ, *et al.*, *Phys. Rev. B* **97**, 085421 (2018).
  - [9] B. Hetényi, C. Kloeffer, D. Loss, *Phys. Rev. Research* **2**, 033036 (2020).
  - [10] E. Knill, *et al.*, *Phys. Rev. A* **77**, 012307 (2008).
  - [11] J. Yoneda, *et al.*, *Nature Nanotechnology* **13**, 102 (2018).
  - [12] K. W. Chan, *et al.*, *Phys. Rev. Applied* **10**, 044017 (2018).
  - [13] J. T. Muhonen, *et al.*, *Nat. Nanotech.* **9**, 986 (2014).
  - [14] W. I. L. Lawrie, *et al.*, *Nano Lett.* (2020).
